# Supplementary material for: Exchange-correlation magnetic fields in spin-density-functional theory
Source: arXiv:1907.08724 ancillary file (2019-07-19)
Supplement: Supplementary file 1 [file Supplemental.pdf]

# Supplemental material for: Exchange-correlation magnetic fields in spin-density-functional theory

Edward A. Pluhar III and Carsten A. Ullrich
*Department of Physics and Astronomy, University of Missouri, Columbia, Missouri 65211, USA*
(Dated: July 19, 2019)

## I. LATTICE HAMILTONIANS WITH $C_2$ SYMMETRY

In the main paper, we consider situations where Hubbard chains are subject to noncollinear magnetic fields. In general, the magnetic fields can have arbitrary magnitude and direction on the different lattice sites; however, it is convenient to look at cases where certain symmetries are present. We wish to investigate here how the symmetries of the magnetic field and of the resulting magnetization are related in a special case.

Let us consider a $P$-point lattice, where $P$ is an even number (the case where $P$ is odd will lead to similar findings, as will be briefly discussed at the end of this Section). We assume, for now, that the system is noninteracting (i.e., $U_0 = U_1 = 0$), and we write the single-particle wave functions as vectors of length $2P$:

$$\mathbf{\Psi} = \begin{pmatrix} \psi_{1\uparrow} \\ \psi_{1\downarrow} \\ \psi_{2\uparrow} \\ \psi_{2\downarrow} \\ \vdots \\ \psi_{P\uparrow} \\ \psi_{P\downarrow} \end{pmatrix} , \tag{1}$$

where $\psi_{k\uparrow,\downarrow}$ are the spin-up and -down components of $\mathbf{\Psi}$ on the $k$th lattice point. The $x, y, z$-components of the magnetization vector on the $k$th lattice site are

$$m_{i,k} = (\psi^*_{k\uparrow}, \psi^*_{k\downarrow})\, \sigma_i \begin{pmatrix} \psi_{k\uparrow} \\ \psi_{k\downarrow} \end{pmatrix} , \qquad k = 1, \ldots, P , \tag{2}$$

where $\sigma_i$ are the Pauli matrices, with $i = x, y, z$.

The (noninteracting) Hamiltonian which determines $\mathbf{\Psi}$ is a $2P \times 2P$ matrix of the form

$$\begin{aligned} \underline{\underline{H}} &= \underline{\underline{T}} + \underline{\underline{V}} + \underline{\underline{B}} \\ &= -[\mathrm{diag}_{+1}(t) + \mathrm{diag}_{-1}(t)] \otimes \sigma_0 \\ &+ \mathrm{diag}(V_1, \ldots, V_P) \otimes \sigma_0 \\ &+ \sum_{i=x,y,z} \mathrm{diag}(B_{i1}, \ldots, B_{iP}) \otimes \sigma_i . \end{aligned} \tag{3}$$

Here, $\mathrm{diag}(a_1, \ldots, a_P)$ denotes a $P \times P$ matrix with the diagonal elements $a_1, \ldots, a_P$ and all other elements zero; $\mathrm{diag}_{\pm 1}(t)$ denotes a matrix where the first upper/lower off-diagonal elements all have the value $t$. $\sigma_0$ is the $2 \times 2$ unit matrix, and $\otimes$ denotes the Kronecker product.

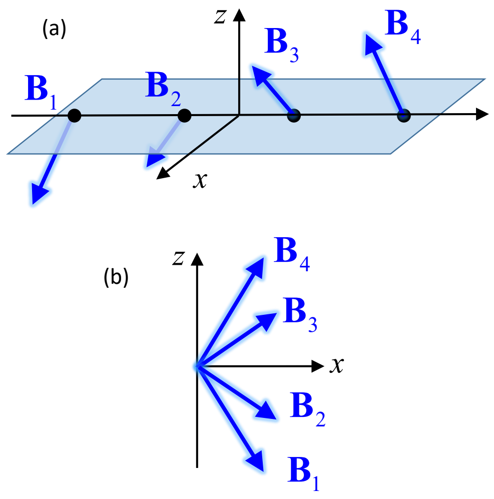


FIG. 1. (a) Example of a magnetic field with $C_2$ symmetry on a 4-point lattice. (b) View along the $y$-axis.

The Hamiltonian matrix (3) has a block-tridiagonal form, where each diagonal block is $2 \times 2$ in size and contains the scalar potentials and magnetic fields on the respective lattice sites. The off-diagonal blocks are $2 \times 2$ unit matrices multiplied by the hopping parameter $-t$.

Now consider a unitary transformation described by a matrix $\underline{\underline{M}}$, which transforms the Schrödinger equation into

$$\underline{\underline{M}}\,\underline{\underline{H}}\,\underline{\underline{M}}^{-1}\underline{\underline{M}}\mathbf{\Psi} = E\underline{\underline{M}}\mathbf{\Psi} . \tag{4}$$

We want to determine how this transformation affects the magnetization (2) for cases of special symmetry. Specifically, we consider scalar potentials that are symmetric about the lattice midpoint, i.e.,

$$V_k = V_{P-k+1} . \tag{5}$$

In the following, we limit ourselves to coplanar magnetic fields; to be specific, we consider magnetic fields in the $x - z$ plane. Assuming that the lattice is aligned along the $y$-direction, we impose $C_2$ symmetry with respect to rotation about the $x$-axis; an example is given in Fig. 1.

$C_2$ symmetric magnetic fields are characterized by the two conditions

$$B_{x,k} = B_{x,P-k+1} , \tag{6}$$
$$B_{z,k} = -B_{z,P-k+1} . \tag{7}$$

This suggests the following transformation matrix:

$$\underline{\underline{M}} = \begin{pmatrix} \underline{0} & \dots & \sigma_x \\ \vdots & \iddots & \vdots \\ \sigma_x & \dots & \underline{0} \end{pmatrix}, \tag{8}$$

which satisfies $\underline{\underline{M}} = \underline{\underline{M}}^\dagger = \underline{\underline{M}}^{-1}$. We need to show that this operator leaves the Hamiltonian (3) invariant, i.e.,

$$\underline{\underline{M}}\,\underline{\underline{H}}\,\underline{\underline{M}}^{-1} = \underline{\underline{H}}\,. \tag{9}$$

The invariance of $\underline{\underline{V}}$ and $\underline{\underline{T}}$ follows immediately from

$$\sigma_x \sigma_0 \sigma_x = \sigma_0\,. \tag{10}$$

For the invariance of $\underline{\underline{B}}$, the transformation must comply with the $C_2$ symmetry of the magnetic field. This follows immediately from

$$\sigma_x \sigma_x \sigma_x = \sigma_x \tag{11}$$

$$\sigma_x \sigma_z \sigma_x = -\sigma_z\,. \tag{12}$$

To calculate the magnetization, we insert the transformed eigenfunction, $\underline{\underline{M}}\mathbf{\Psi}$, into Eq. (2), where

$$\underline{\underline{M}}\mathbf{\Psi} = \begin{pmatrix} \psi_{P\downarrow} \\ \psi_{P\uparrow} \\ \vdots \\ \psi_{1\downarrow} \\ \psi_{1\uparrow} \end{pmatrix}. \tag{13}$$

This gives the final result

$$m_{x,k} = m_{x,P-k+1} \tag{14}$$

$$m_{z,k} = -m_{z,P-k+1}\,. \tag{15}$$

In other words, the magnetization also has $C_2$ symmetry, as expected.

We conclude this Section with three remarks.

1. If the number of lattice sites $P$ is odd, $C_2$ symmetry requires that in the central site the magnetic field and the magnetization point along the $x$-direction. The definition of $\underline{\underline{M}}$ must be recast by putting $\sigma_0$ as the central block of $\underline{\underline{M}}$. The proof then goes through as before.

2. The symmetry property of the magnetization, Eqs. (14) and (15), remains intact when interactions are present. This is because the Hamiltonian of the interacting system remains invariant under $C_2$ symmetry transformations. This implies that the Kohn-Sham system also has a magnetization which satisfies conditions (14) and (15), which is intuitively clear since the exchange-correlation magnetic field is evaluated self-consistently with a magnetization of the $C_2$ symmetry type. Our numerical results confirm this.

3. Here, we considered $C_2$ symmetry with respect to rotations about the $x$-axis, which made the proof simpler. In the main paper, the lattice Hamiltonian has $C_2$ symmetry with respect to rotations about an axis that lies at a 45° angle between the $x$ and the $z$ axis. Equations (14) and (15) then turn into the single condition

$$m_{x,k} = m_{z,P-k+1}\,. \tag{16}$$

## II. INVERTING THE KOHN-SHAM EQUATION IN NONCOLLINEAR SPIN-DFT

The inverse problem in Kohn-Sham density-functional theory (KS DFT) can be stated as follows: what is the local effective potential which generates a given density as the ground-state density of a KS system? Often, the given density is the exact (or highly accurate) density of a many-body system in a prescribed external potential, which was obtained by other means (such as highly accurate and expensive many-body techniques); by inversion, one can then construct the exact exchange-correlation (xc) potential associated with this density. The exact xc potential can then be compared with approximations. There are various numerical techniques to reverse-engineer the KS potential for a given density, as reviewed by Jensen and Wasserman [1].

Here, the task is to construct that KS system which reproduces a target 4-density $\vec{m}_k^t$, $k = 1, \dots, P$, on a $P$-site Hubbard chain, where the 4-vector notation $\vec{m}_k^t = (n_k, \mathbf{m}_k)$ means that the zeroth component is the scalar density (or site occupation), followed by the three components of the magnetization on site $k$. This vector notation was introduced in Ref. [2].

The KS system which reproduces $\vec{n}_k^{(t)}$ is characterized by a 4-potential $\vec{v}_{\mathrm{KS},k} = (V_{\mathrm{KS},k}, \mathbf{B}_{\mathrm{KS},k})$, $k = 1, \dots, P$, where the zeroth component is the KS scalar potential and the remaining three components are the KS magnetic field [2].

Once the target 4-density $\vec{m}_k^t$ has been calculated via exact diagonalization of the interacting Hamiltonian, we define an iterative procedure to construct $\vec{v}_{\mathrm{KS},k}$ by means of a cost functional $F[\vec{v}_{\mathrm{KS}}^{(i)}]$, where the superscript denotes the $i$th iteration step:

$$F[\vec{v}_{\mathrm{KS}}^{(i)}] = \sum_{k=1}^{P} \left| \vec{m}_k^{(i)}[\vec{v}_{\mathrm{KS}}^{(i)}] - \vec{m}_k^t \right|^2 . \tag{17}$$

This cost functional is positive definite, and, thanks to the Hohenberg-Kohn theorem, there is a single, unique minimum that occurs when $\vec{m}_k^{(i)}$, the density configuration in the $i$th iteration step, agrees with the target density $\vec{m}_k^t$. At the minimum, the cost functional has the value zero. In practice, the search is declared a success when the value of $F$ falls below an appropriately chosen small threshold.

To implement a conjugate gradient (CG) search algorithm [3], we need the derivative of the cost functional:

$$\frac{\partial F}{\partial v_{\mathrm{KS},jq}^{(i)}} = \sum_{k=1}^{P} 2\left(\vec{m}_k^{(i)} - \vec{m}_k^t\right) \cdot \frac{\partial \vec{m}_k^{(i)}}{\partial v_{\mathrm{KS},jq}}\,, \tag{18}$$

where the index $j$ runs over all $P$ lattice sites, and the index $q = 0, 1, 2, 3$ runs over the 4 components of $\vec{v}_{\mathrm{KS},j}$.

We have

$$\vec{m} = \begin{pmatrix} m_0 \\ m_1 \\ m_2 \\ m_3 \end{pmatrix} = \begin{pmatrix} n_{\uparrow\uparrow} + n_{\downarrow\downarrow} \\ n_{\uparrow\downarrow} + n_{\downarrow\uparrow} \\ i(n_{\uparrow\downarrow} - n_{\downarrow\uparrow}) \\ n_{\uparrow\uparrow} - n_{\downarrow\downarrow} \end{pmatrix}, \qquad (19)$$

where the KS spin-density matrix follows by summing over the occupied KS orbitals:

$$\begin{pmatrix} n_{\uparrow\uparrow} & n_{\uparrow\downarrow} \\ n_{\downarrow\uparrow} & n_{\downarrow\downarrow} \end{pmatrix} = \sum_{a=1}^{\rm occ} \begin{pmatrix} |\psi_{a\uparrow}|^2 & \psi_{a\uparrow}\psi_{i\downarrow}^* \\ \psi_{a\downarrow}\psi_{i\uparrow}^* & |\psi_{a\downarrow}|^2 \end{pmatrix}. \qquad (20)$$

Hence, to evaluate $\partial \vec{m}_k^{(i)}/\partial v_{\mathrm{KS},jq}$ in Eq. (18), we need derivatives of the KS spin orbitals with respect to $v_{\mathrm{KS},jb}$. These can be obtained from first-order perturbation theory:

$$\frac{\partial \psi_{a\sigma,k}}{\partial v_{\mathrm{KS},jq,k'}} = \sum_{b\neq a} \frac{\Psi_{b,k'}^\dagger \sigma_q \Psi_{a,k'}}{\epsilon_a - \epsilon_b}\, \psi_{b\sigma,k}\ , \qquad (21)$$

where $\epsilon_a$ and $\epsilon_b$ are KS energy eigenvalues, and $\Psi_{b,k'}^\dagger = (\psi_{b\uparrow,k'}^*, \psi_{b\downarrow,k'}^*)$.

The ingredients of the CG algorithm to minimize the cost function are now all in place. As stated, we begin from an exact target solution, and then solve the KS equation for a given initial condition. The corresponding KS density and magnetizations are fed into the CG routine, where the cost functional and gradients are calculated. After finding a step direction, the KS equation is recalculated at the new configuration space site, where the new density and magnetization can be used to continue convergence.

It is difficult to find a global minimum in general, and the CG method we employ is no different. In our research, we have found that $\lambda = F \leq 10^{-16}$ calculates density and magnetization values to within $10^{-7}$ of $\vec{m}_k^t$, where $\lambda$ is our threshold for convergence. Occasionally, the CG routine will approach a local minimum that is greater than $\lambda$. When such an occurrence happens, we systematically select new initial conditions for our KS density and magnetizations. After calculating and converging to an optimized $\vec{m}_k$ for the initial choice of $U_0$ (which is generally $U_0 = 0$), we restart the following iteration from the final converged $\vec{m}_k$ that matched $\vec{m}_k^t$ to within $\lambda$ of our cost function.

As seen in Fig. 2, we can have convergence to a local minimum even after a restarted calculation. In such events, we step away from our initial potential in increasing increments in all directions in the potential space, governed by a step size, $\delta_k$. Once a minimum meeting our threshold is found, the step search terminates and the xc potentials and magnetic fields (giving rise to the xc torques) are then calculated from the final potential.

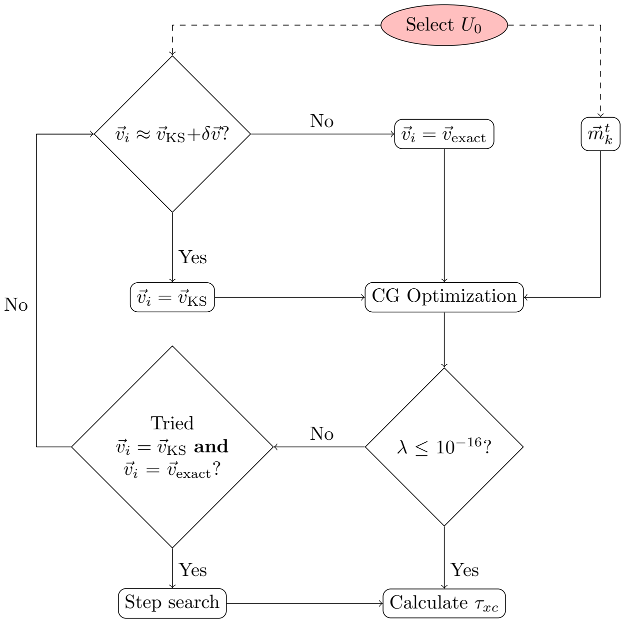


FIG. 2. Flow chart of the conjugate gradient routine used to calculate the exact xc potentials and magnetic fields (giving rise to the xc torques $\tau_{\rm xc}$).

## III. ENFORCING THE ZERO-TORQUE THEOREM

The zero-torque theorem states that the xc magnetic field cannot exert a net torque on the system itself [4]. While this is true for the exact xc magnetic field, a given approximation may violate this requirement, so that

$$\int d\mathbf{r}\, \mathbf{m}(\mathbf{r}) \times \mathbf{B}_{\rm xc}^{\rm app}(\mathbf{r}) = \mathbf{T}\ , \qquad (22)$$

where $\mathbf{T}$ is a spurious macroscopic torque.

Kurzweil, Baer and Head-Gordon [5, 6] showed how to enforce exact conditions on approximate local xc potentials by using constrained minimization with Lagrange multipliers. Here, we use a similar approach (but without Lagrange multipliers) to enforce the zero-torque theorem. The idea is to construct a counteracting field $\mathbf{b}(\mathbf{r})$ such that

$$\int d\mathbf{r}\, \mathbf{m}(\mathbf{r}) \times \mathbf{b}(\mathbf{r}) = \mathbf{T} \qquad (23)$$

and

$$||\mathbf{b}(\mathbf{r})||^2 \equiv \int d\mathbf{r} |\mathbf{b}(\mathbf{r})|^2 = \min. \qquad (24)$$

In other words, we are looking for a vector field which generates the same macroscopic torque, but whose integrated vector norm is as small as possible. Once such a $\mathbf{b}(\mathbf{r})$ has been found, we define

$$\tilde{\mathbf{B}}_{\rm xc}^{\rm app}(\mathbf{r}) = \mathbf{B}_{\rm xc}^{\rm app}(\mathbf{r}) - \mathbf{b}(\mathbf{r}) \qquad (25)$$

as a new approximation, which now satisfies the zero-torque theorem while remaining as close as possible to the original $\mathbf{B}_{\rm xc}^{\rm app}(\mathbf{r})$. We now show how to explicitly find $\mathbf{b}(\mathbf{r})$ on a lattice, distinguishing two cases.

### A. Coplanar case

We consider a $P$-point lattice where the magnetization and the xc magnetic field are in the $x-z$ plane everywhere. All torques are therefore in the $y$-direction only. Equation (23) for the $\mathbf{b}$-field then becomes

$$\sum_{i=1}^{P}[m_{zi}b_{xi} - m_{xi}b_{zi}] = T_y \ . \tag{26}$$

We can rewrite this as

$$b_{zP} = \frac{1}{m_{xP}}\sum_{i=1}^{P-1}[m_{zi}b_{xi} - m_{xi}b_{zi}] + \frac{m_{zP}b_{xP}}{m_{xP}} - \frac{T_y}{m_{xP}} \tag{27}$$

and in this way express $b_{zP}$ as a function of all other $b_{xk}$ $(k = 1,\dots,P)$ and $b_{zj}$ $(j = 1,\dots,P-1)$.

The integrated vector norm of $\mathbf{b}$ on the lattice is

$$||\mathbf{b}||^2 = \sum_{i=1}^{P}(b_{xi}^2 + b_{zi}^2). \tag{28}$$

To minimize this, we calculate the partial derivatives

$$\begin{aligned}\frac{1}{2}\frac{\partial||\mathbf{b}||^2}{\partial b_{xk}} &= b_{xk} + \frac{m_{zk}}{m_{xP}}b_{zP}\\ \frac{1}{2}\frac{\partial||\mathbf{b}||^2}{\partial b_{zj}} &= b_{zj} - \frac{m_{xj}}{m_{xP}}b_{zP} \ ,\end{aligned}$$

where we used Eq. (27). Setting the derivatives equal to zero gives

$$\begin{aligned}m_{xP}b_{xk} &= -m_{zk}b_{zP}\\ m_{xP}b_{zj} &= m_{xj}b_{zP}\end{aligned}$$

and we can rewrite this, using Eq. (27), as

$$\begin{aligned}m_{xP}^2 b_{xk} &= -m_{zk}\sum_{i=1}^{P-1}(\mathbf{m}_i\times\mathbf{b}_i)_y - m_{zk}m_{zP}b_{xP} + m_{zk}T_y\\ m_{xP}^2 b_{zj} &= m_{xj}\sum_{i=1}^{P-1}(\mathbf{m}_i\times\mathbf{b}_i)_y + m_{xj}m_{zP}b_{xP} - m_{xj}T_y \ .\end{aligned}$$

It is straightforward to see that this is solved by

$$\mathbf{b}_i = \frac{\mathbf{T}\times\mathbf{m}_i}{\sum_{l=1}^{P} m_l^2} \ . \tag{29}$$

The same argument can be repeated for the $x-y$ and $y-z$ planes. Thus, in the coplanar case we find that

$$\tilde{\mathbf{B}}_{{\rm xc},i}^{\rm app} = \mathbf{B}_{{\rm xc},i}^{\rm app} - \frac{\mathbf{T}\times\mathbf{m}_i}{\sum_{l=1}^{P} m_l^2} \tag{30}$$

is the zero-force-theorem corrected xc magnetic field as close as possible to the original one.

### B. General case

In the general case where the magnetization and xc magnetic field are not constrained to be in the same plane everywhere, a simple analytic expression for $\mathbf{b}_i$ is unfortunately not available; instead, $\mathbf{b}_i$ must be determined numerically.

For a $P$-point lattice, Eq. (23) becomes

$$\mathbf{T} = \sum_{i=1}^{P}\mathbf{m}_i\times\mathbf{b}_i \ , \tag{31}$$

and we can rewrite this as

$$\mathbf{m}_P\times\mathbf{b}_P = -\sum_{i=1}^{P-1}\mathbf{m}_i\times\mathbf{b}_i + \mathbf{T} \ . \tag{32}$$

From this vector equation we can find explicit expressions for two variables, say $b_{yP}$ and $b_{zP}$:

$$b_{yP} = \frac{1}{m_{xP}}\sum_{i=1}^{P-1}(m_{yi}b_{xi} - m_{xi}b_{yi}) + \frac{m_{yP}}{m_{xP}}b_{xP} + \frac{T_z}{m_{xP}} \tag{33}$$

$$b_{zP} = \frac{1}{m_{xP}}\sum_{i=1}^{P-1}(m_{zi}b_{xi} - m_{xi}b_{zi}) + \frac{m_{zP}}{m_{xP}}b_{xP} - \frac{T_y}{m_{xP}} \ . \tag{34}$$

Furthermore, the right-hand side of Eq. (32) must be perpendicular to $\mathbf{m}_P$:

$$\mathbf{m}_P\cdot\left[\sum_{i=1}^{P-1}\mathbf{m}_i\times\mathbf{b}_i - \mathbf{T}\right] = 0 \ , \tag{35}$$

and we can use this to find an explicit expression for another variable, say $b_{x1}$:

$$b_{x1} = \frac{\mathbf{m}_P\cdot\mathbf{T}}{(\mathbf{m}_P\times\mathbf{m}_1)_x} + b_{y1}a_{y1} + b_{z1}a_{z1} + \sum_{i=2}^{P-1}\mathbf{b}_i\cdot\mathbf{a}_i \tag{36}$$

where

$$\mathbf{a}_i = -\frac{\mathbf{m}_P\times\mathbf{m}_i}{(\mathbf{m}_P\times\mathbf{m}_1)_x} \ . \tag{37}$$

The integrated vector norm of $\mathbf{b}$ on the lattice is

$$||\mathbf{b}||^2 = \sum_{i=1}^{P}(b_{xi}^2 + b_{yi}^2 + b_{zi}^2). \tag{38}$$

In this expression, we eliminate $b_{x1}$, $b_{yP}$ and $b_{zP}$ using Eqs. (36), (33) and (34); this means that $||\mathbf{b}||^2$ contains $3P-3$ independent variables, namely, $b_{x2},\dots,b_{xP}$, $b_{y1},\dots,b_{yP-1}$, and $b_{z1},\dots,b_{zP-1}$. Setting the derivatives of $||\mathbf{b}||^2$ with respect to each of these variables equal to zero leads to a system of $3P-3$ linear equations, which can be numerically solved with standard methods. Together with Eqs. (36), (33) and (34) this then yields all components of $\mathbf{b}_i$ on all lattice points.

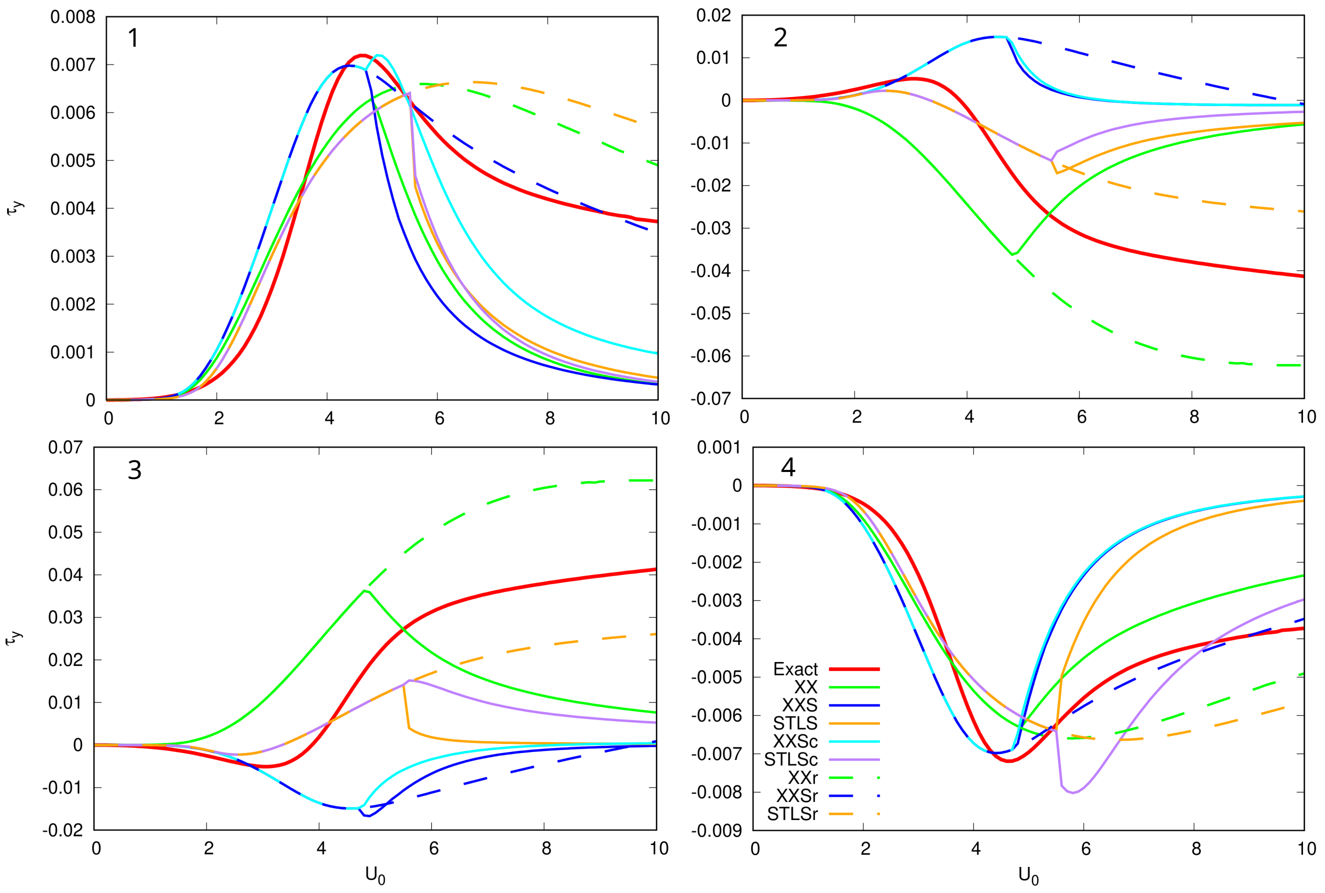


FIG. 3. $\tau_{\rm xc}$'s for $C_2$ symmetric system with torque corrections. Torque corrections are only required after the system spontaneously breaks symmetry, as the solutions satisfy the zero-torque theorem prior to breaking symmetry.

## IV. ADDITIONAL NUMERICAL RESULTS FOR THE HUBBARD TETRAMERS

Figure 3 shows the xc torques on the four sites the $C_2$-symmetric lattice. In addition to the results shown in Fig. 13 in the main paper, we also include the torque-corrected results. The zero-torque theorem is satisfied for the symmetry-restricted case, so the torque-corrected results are only relevant once the $C_2$-symmetry is broken. Some differences between the XXS and XXSc results and between the STLS and STLSc results can be observed, but the xc torque correction has no impact on the symmetry breaking.

Next, to assess the significance of the xc torques, we have performed self-consistent calculations in which only the longitudinal component of the xc magnetic field is included, defined as

$$\mathbf{B}_{\rm xc,||} = \frac{(\mathbf{m}\cdot\mathbf{B}_{\rm xc})\mathbf{m}}{m^2} \ . \tag{39}$$

Figures 4 and 5 show the $x$- and $z$-components of the magnetization of the nonsymmetric tetramer, and Figs. 6 and 7 show the same for the $C_2$-symmetric tetramer, comparing the exact results, the Kohn-Sham results with the full $\mathbf{B}_{\rm xc}$, and the Kohn-Sham results with the longitudinal $\mathbf{B}_{\rm xc}$ (dashed lines).

Overall, the differences between the full calculations and the longitudinal-only calculations are mostly minor, except for XX, see below. In the nonsymmetric case, the biggest relative deviations are on sites 3 and 4 for the $x$-component and on site 1 for the $z$-component; however, on these sites, the respective components of magnetization are small to begin with.

The same is the case for the $C_2$-symmetric lattice, at least for XXS and STLS. For XX, on the other hand, the longitudinal restriction causes some major differences for the unrestricted solution, and seems to push the symmetry breaking along opposite directions. Some differences, although less pronounced, also appear for the symmetry-restricted XX solutions, which now are closer to the XXS and STLS solutions. It is not obvious why the XX appears to be more sensitive to the presence of transverse magnetic fields, but it is clearly related to the fact that XX produces larger xc torques than XXS and STLS.

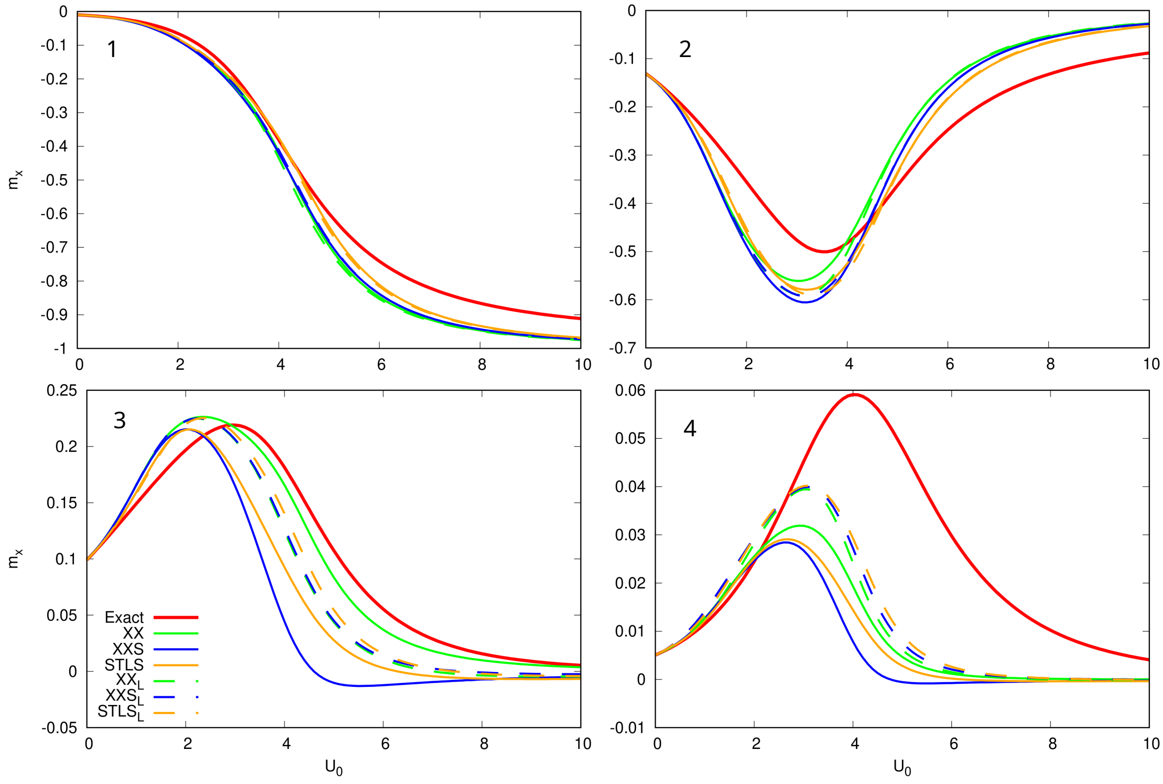


FIG. 4. $x$-component of the magnetization for the nonsymmetric lattice, comparing exact results, Kohn-Sham results with the full $\mathbf{B}_{\rm xc}$, and Kohn-Sham results with the longitudinal $\mathbf{B}_{\rm xc}$ (dashed lines).

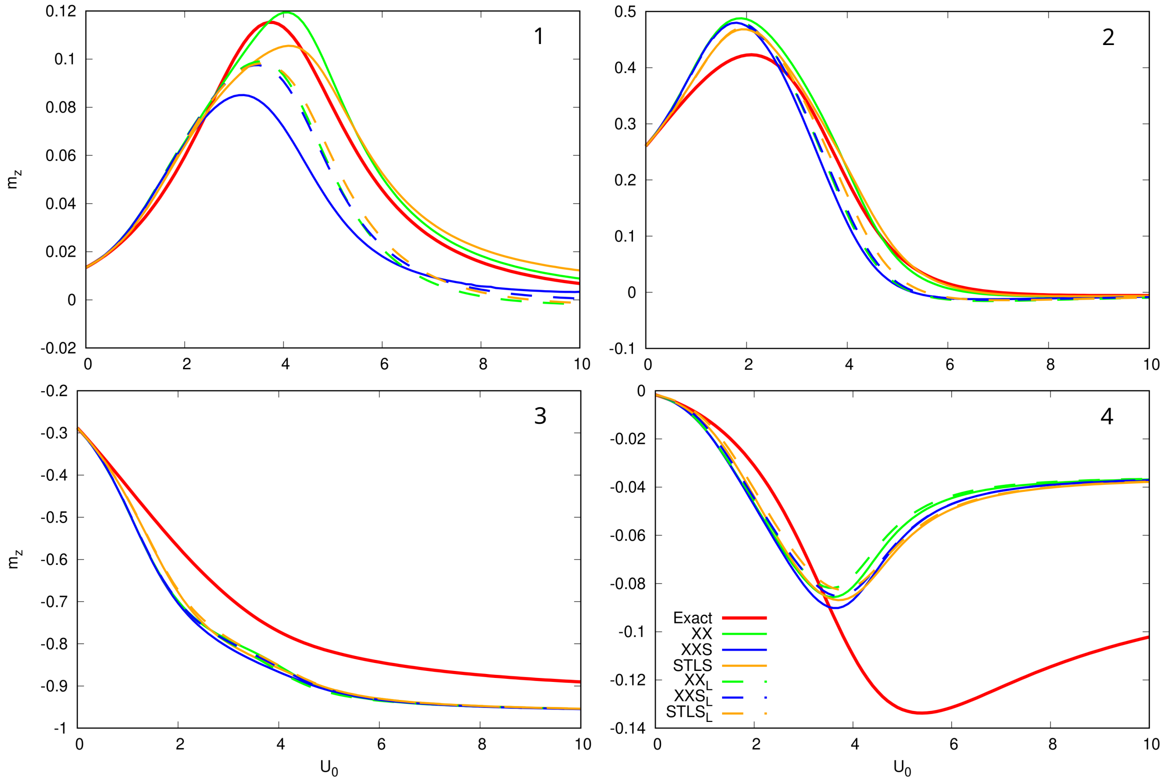


FIG. 5. Same as Fig. 4, but for $m_{z,k}$.

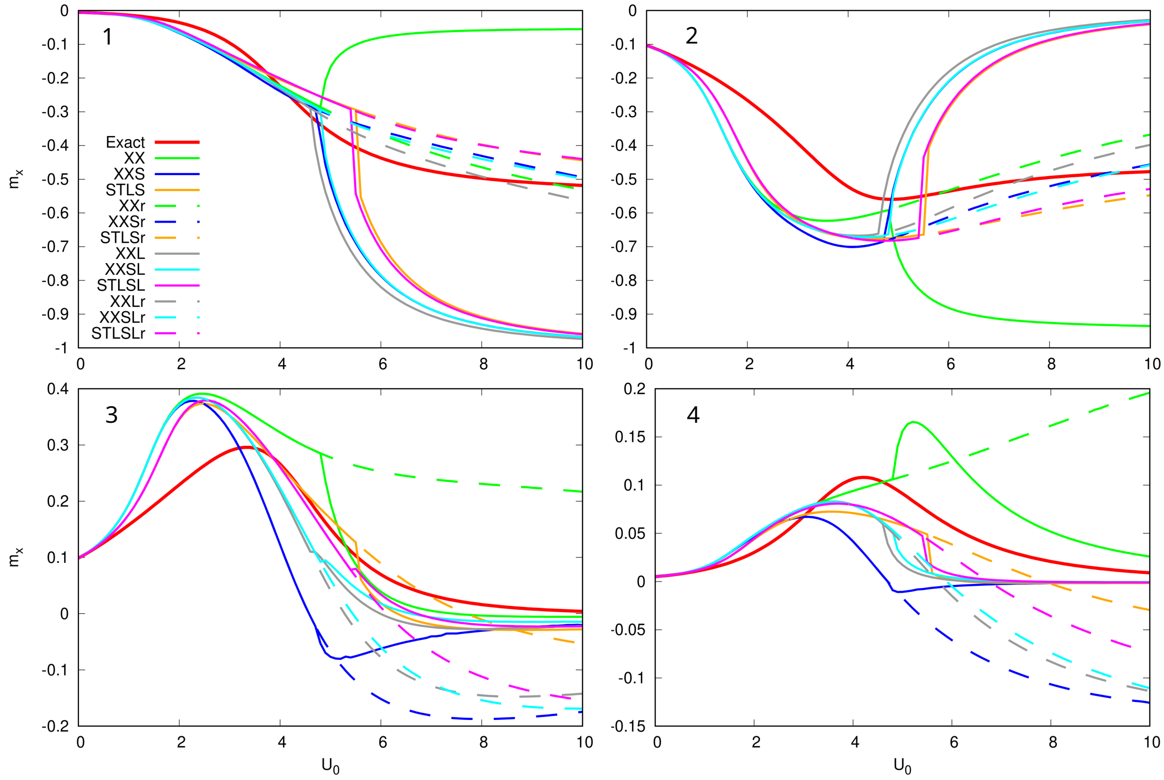


FIG. 6. Same as Fig. 4, but for the $C_2$-symmetric lattice.

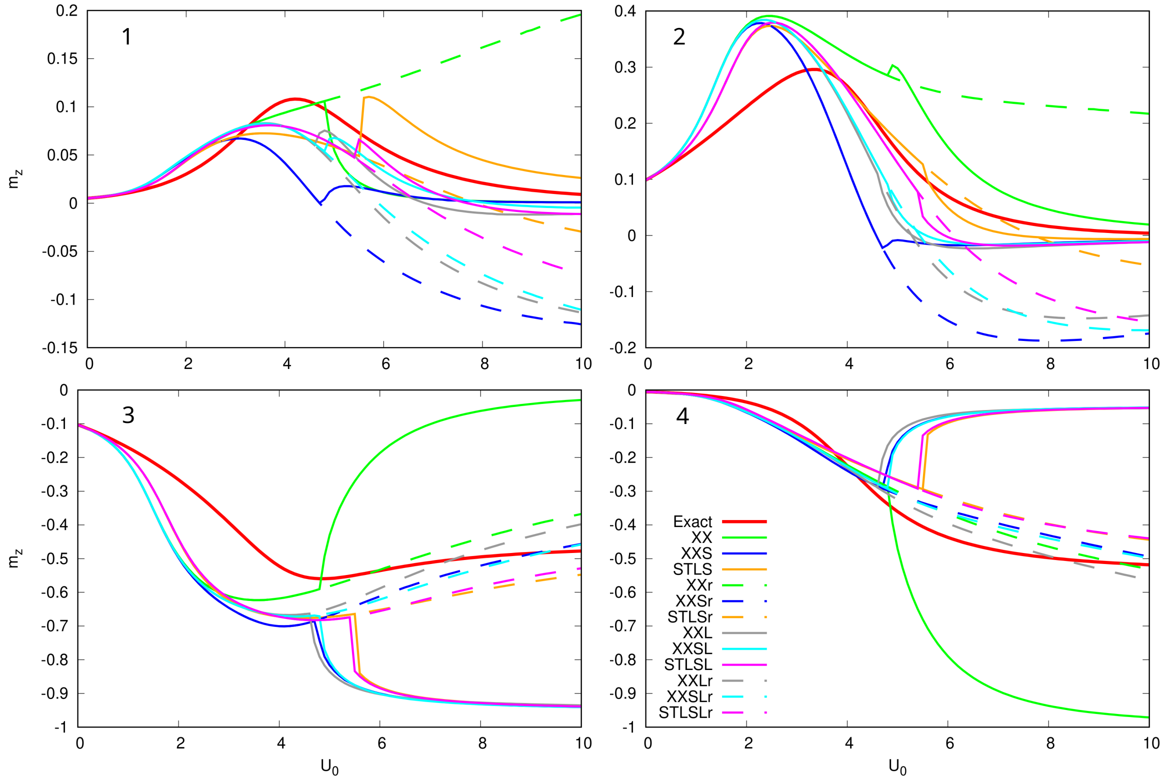


FIG. 7. Same as Fig. 5, but for the $C_2$-symmetric lattice.

[1] D. S. Jensen and A. Wasserman, Numerical methods for the inverse problem of density functional theory, Int. J. Quant. Chem. **118**, e25425 (2017).
[2] C. A. Ullrich, Density-functional theory for systems with noncollinear spin: orbital-dependent exchange-correlation functionals and their application to the Hubbard dimer, Phys. Rev. B **98**, 035140 (2018).
[3] W. H. Press, S. A. Teukolsky, W. T. Vetterling, and B. P. Flanner, *Numerical recipes 3rd edition: the art of scientific computing* (Cambridge University Press, Cambridge, 2007).
[4] K. Capelle, G. Vignale, and B. L. Györffy, Spin currents and spin dynamics in time-dependent density-functional theory, Phys. Rev. Lett. **87**, 206403 (2001).
[5] Y. Kurzweil and R. Baer, Adapting approximate-memory potentials for time-dependent density functional theory, Phys. Rev. B **77**, 085121 (2008).
[6] Y. Kurzweil and M. Head-Gordon, Improving approximate-optimized effective potentials by imposing exact conditions: Theory and applications to electronic statics and dynamics, Phys. Rev. A **80**, 012509 (2009).
